# Supplementary material for: A New Dynamic Algorithm for Densest Subhypergraphs
Source: arXiv:2204.08106 source file (2022-04-17)
Supplement: Supplementary file 1 [file supplement.tex]

\section{Additional Experimental Details}
\label{sec:appendix:exp}
